# Supplementary material for: LocAgent: Graph-Guided LLM Agents for Code Localization
Source: arXiv:2503.09089 source file (2025-04-29)
Supplement: Supplementary file 1 [file 6_2_appendix_graph.tex]

\section{Code Graph Construction Details}
\subsection{Analysis of computational complexity}
In the following, we analyze the computational complexity of building code graphs for codebases.

(1) \textit{The sizes of code graphs for codebases are relatively small.}
We set the smallest node granularity of our code graphs as functions. Consequently, the graph remains manageable even for large repositories. For example, the largest codebase in SWE-bench lite contains only 45k nodes and 430k edges.

(2) \textit{The computational complexity of graph construction increases linearly with the graph size.}
Given a code graph, let $N$ denote the total number of nodes and $M$ denote the total number of edges. Our graph construction involves the following steps:

\begin{itemize}
    \item Using the codebase's natural tree structure, we perform depth-first search to collect nodes and "contain" edges, with time complexity $O(N)$.
    \item We collect "import" edges (i.e., file → file/class/function) for all files with time complexity $O(M_{\text{import}})$, where $M_{\text{import}}$ represents the number of these edges.
    \item For collecting "invoke" and "inherit" edges that originate from functions or classes, we must identify all candidate target functions/classes within their callable scope:
        (a) We analyze the modules imported by each file, noting that a single import edge may grant access to multiple functions or classes. Let $d_{\text{import}}$ represent the average number of functions or classes available per import edge. Under this formulation, identifying potential imported candidates exhibits a time complexity of $O(M_{\text{import}} \cdot d_{\text{import}})$.
        
        (b) We examine the callable scope for each function or class. The Python files form a hierarchical tree where $l_{\text{file-depth}}$ represents average tree depth and $d_{\text{contain}}$ represents average children per node. For each function/class, we recursively traverse its parent node to collect candidates. With $N_{\text{func}}$ functions and $N_{\text{class}}$ classes, identifying candidates within the file has time complexity $O((N_{\text{func}} + N_{\text{class}}) \cdot l_{\text{file-depth}} \cdot d_{\text{contain}})$.

    \item Finally, we traverse each function/class's abstract syntax tree (AST) to collect "invoke" and "inherit" edges. We match the target nodes within the candidate set. With $d_{\text{func-ast}}$ representing the average number of AST nodes within each function (excluding inner functions/classes), this has time complexity $O((N_{\text{func}} + N_{\text{class}}) \cdot d_{\text{func-ast}})$.
\end{itemize}

Since $N_{\text{func}} + N_{\text{class}} \approx N$, the overall time complexity simplifies to $O(N \cdot (d_{\text{func-ast}} +l_{\text{file-depth}} \cdot  d_{\text{contain}}) + M_{\text{import}} \cdot d_{\text{import}})$. This linear relationship with graph size enables efficient updates when modifying nodes and edges.

\subsection{Analysis of indexing latency}
We present a comparison of indexing latency and resource usage across different methods in table below.
% \begin{table}[ht!]
%     \centering
%     \small
%     \resizebox{\linewidth}{!}{%
%     \begin{tabular}{lcccc}
%         \toprule
%         % Method & Index Time (s) & Retrieval Time (s) & Total Time (s) \\
%         % \midrule
%         % BM25 & - & - & - \\
%         % CodeSage-Large & - & - & - \\
%         % CodeT5+ & - & - & - \\
%         % Jina-Code-v2 & - & - & - \\
%         % CodeRankEmbed & - & - & - \\
%         \textbf{Method} & \textbf{Param.} & \textbf{Index Time (s)} & \textbf{Retrieval Time (s)} & \textbf{Memory Footprint (GB)} \\
%         \midrule
%         BM25 & - & - & - & - \\
%         e5-base & 110M & 34 & 5.4 & 4 \\
%         e5-base-v2 & 110M & 34 & 5.4 & 4 \\
%         CodeSage-Large & 1.3B & 34 & 81 & 41 \\
%         Codesage-large-v2 & 1.3B & 34 & 83 & 41 \\
%         CodeT5+ & 110M & 34 & 23.5 & 13 \\
%         Jina-Code-v2 & 161M & 34 & 13 & 28 \\
%         CodeRankEmbed & 137M & 34 & 15 & 24 \\
%         % SFR-Embedding-Mistral & 7B & 34 & 138 & 77 \\
%         \midrule
%         Agentless & - & - & - \\
%         openhands & - & - & - \\
%         moatless & - & - & - \\
%         Ours & - & - & - \\
%         \bottomrule
%     \end{tabular}
%     }
%     \caption{Computational efficiency comparison of different code indexing methods.}
%     \label{tab:time_efficiency}
% \end{table}

\begin{table}[h!]
\centering
\resizebox{\linewidth}{!}{%
\begin{tabular}{lllrr}
\toprule
\textbf{Method}          & \textbf{Device} & \textbf{Parallelism} & \makecell[c]{\textbf{Latency} \\ \textbf{per repo}} & \textbf{Total time} \\ \midrule \midrule
\textsc{LocAgent}                & CPU             & repo-level           & 587s                           & 0.9h                     \\ 
E5-base-v2              & GPU             & chunk-level          & 45s                            & 1.2h                     \\ 
Jina-Code-v2            & GPU             & chunk-level          & 53s                            & 1.8h                     \\ 
Codesage-large-v2       & GPU             & chunk-level          & 123s                           & 7h                       \\ 
CodeRankEmbed           & GPU             & chunk-level          & 55s                            & 1.9h                     \\ \bottomrule
\end{tabular}
}
\caption{Time efficiency comparison of different code indexing methods.}
\label{tab:time_efficiency}
\end{table}

While our current graph construction process is not yet fully optimized, it already demonstrates reasonable overall time efficiency. The relatively high per-repository latency is due to a Python-based, repo-level parallel implementation that utilizes only a single CPU core per repo. However, with such embarrassing parallel, we can achieve high throughput across repositories (we use 50 parallel processes here). As a result, the total indexing time remains low despite the higher per-repo latency.

Although vector-based methods benefit from GPU acceleration, they require more compute resources and incur higher total processing time due to heavier model computations. In contrast, \textsc{LocAgent} has significantly lower computational complexity for constructing graph index, which is linear to the graph size, and it achieves better overall efficiency with lower resource requirements.
